# Supplementary material for: NOPE: Novel Object Pose Estimation from a Single Image
Source: arXiv:2303.13612 source file (2024-03-29)
Supplement: Supplementary file 1 [file supp.tex]

\section{Supplementary Material}

\vspace*{-4pt}
\subsection{Ablation study}
\label{sec:ablation}

\vspace*{-2pt}
\paragraph{Pose conditioning. } 
\vspace*{-4pt}
We experimented with two different pose representations. 
3DiM first creates camera rays from a given 3D pose and uses the positional encoding of \cite{mildenhall2020nerf} to obtain a pixel-wise pose condition.  This representation is then processed by an MLP before being integrated into the feature map of the U-Net as in our method. We experimented with this method but discovered it does not improve the performance for our problem compared to applying an MLP directly to a representation of the rotation. We favored the second approach for its simplicity.

% conditioning strategy and discovered that it doesn't enhance accuracy. Our current pose conditioning, on the other hand, is much more straightforward.
\begin{table}[!t]
    \addtolength{\tabcolsep}{-2pt}
    \centering
    \scalebox{0.8}{
    \begin{tabular}{@{}l c c c c @{}}
    \toprule
    Metric & Euler angle & Axis-angle & Quaternion & Rotation-6D~\cite{zhou2019continuity} \\
    \midrule
    Acc30 $\uparrow$ & 74.2 & 74.7 &  75.2 & \bf 75.5 \\
    $\bm{\MedErr}\downarrow$ & \hphantom{0}8.8 & \hphantom{0}8.5 & \bf \hphantom{0}8.1 & \bf \hphantom{0}8.1 \\
    \bottomrule
    \end{tabular}}
    \vspace*{-10pt}
    \caption{{\bf Ablation study of rotation representation} on ``novel instances'' test set. Rotation-6D yields slightly better performance than other representations.}
    % } % when testing on ``novel instances''.}% of training categories.}
    \label{tab:ablation_rotation}
\end{table}

\vspace*{-10pt}
\paragraph{Rotation representation for the relative pose.} 
Similarly, we experimented with different representations for the rotation:  axis-angles, quaternions, and rotation-6D~\cite{zhou2019continuity}. \nguyen{As shown in Table~\ref{tab:ablation_rotation}, rotation-6D~\cite{zhou2019continuity} yields slightly better performances than other representations, so we use this representation in all of our experiments.}

% \vspace*{-35pt}

\subsection{Denoising Diffusion Probabilistic Models (DDPM)}
\paragraph{Diffusion model.}
Diffusion models~\cite{sohl2015deep, ho2020denoising, song2019generative, song2021denoising} are a class of likelihood-based models inspired by nonequilibrium thermodynamics~\cite{song2019generative, song2020improved}. These models define a Markovian chain of diffusion forward process by gradually adding noise to sample data. The forward noise process is defined as
\begin{equation}
\label{eq:noise_process}
    q(\bm{z}_t | \bm{z}_0) = \mathcal{N}(\bm{z}_t | \sqrt{\bar{\alpha}_t} \bm{z}_0, (1 - \bar{\alpha}_t) \bm{I}),
\end{equation}
which transforms data sample $\bm{z}_0$ to a latent noisy sample $\bm{z}_t$ for $t\in\{0, 1, ...,T\}$ by adding noise to $\bm{z}_0$.

$\bar{\alpha}_t \coloneqq \prod_{s=0}^{t} \alpha_s = \prod_{s=0}^{t} (1 - \beta_s)$ and $\beta_s$ represents the noise variance schedule~\cite{ ho2020denoising}.
During training, a neural network $f_\theta(\bm{z}_t, t)$ is trained to predict $\bm{z}_0$ from $\bm{z}_t$ by minimizing the training objective with $\ell_2$ loss~\cite{ho2020denoising}:
\begin{equation}
    \mathcal{L}_\text{train} =  \frac{1}{2}|| f_\theta(\bm{z}_t, t) - \bm{z}_0 ||^2.
\end{equation}
